# Supplementary material for: Private Multi-Winner Voting for Machine Learning
Source: arXiv:2211.15410 source file (2022-11-23)
Supplement: Supplementary file 1 [file appendix_backup.tex]

\section{Optimized Loss for Multi-Label Classification}

For each of our voting schemes, the metrics we use are based on the average per label. Therefore the Hamming loss is optimal and is used to train the teachers. In the case of medical datasets, a partially correct prediction for one sample still has value while the subset 0/1 loss is more strict and requires every label in the prediction for a sample to be equal to the target, therefore not differentiating between \textit{almost correct} and \textit{completely wrong} predictions~\cite{Dembczynski2012OnLD}. Thus, using the subset loss or the subset accuracy as metrics for our tasks is less representative of the situations we deal with. While it is true that for the \powerset method, which is based on the output of all labels, the subset 0/1 loss is more tailored, training a model using the subset 0/1 loss is difficult especially over a large number of labels and a relatively small number of samples (e.g., 20 labels and 5823 samples for the Pascal VOC dataset). Here a large number of labels generates many possible label subsets, called meta-classes (more than 1 million with 20 labels). When we train the teacher models using the standard cross-entropy loss on all these meta-classes, the performance is very poor. We therefore use the binary cross-entropy loss to train the teachers on the multi-label datasets. Furthermore, current literature which uses the subset 0/1 loss in multi-label classification refers to label dependence which was not the focus of our current work. For the \powerset method, after training the teacher models, we reduce the task to the single-label classification so Hamming and 0/1 losses act in the same way. 

%\FloatBarrier
\section{The \capc Protocol}\label{app:capc-protocol}

The \capc protocol is as follows: 

\begin{enumerate}
    \item \textbf{Private inference} is run for each answering party. 
    \begin{enumerate}
        \item \textbf{Compute logits.} A querying party (or, student) sends an encrypted query 
        % (the data point to be labeled) 
        (unlabeled $x$)
        to each answering party (or, teacher). The teachers run the private inference and upon completion return encrypted logits: $Enc(r)$.
        % At the end of this step, teachers have computed logits, which are in an encrypted form: $Enc(r)$.
        \item \textbf{Secret sharing} between the answering and querying parties. Each answering party generates a random vector $\hat{r}$ and subtracts it from the vector of logits $r$. Then, each answering party sends the encrypted result: $Enc(r-\hat{r})$ to the querying party who decrypts the message to obtain $(r-\hat{r})$.
        \item \textbf{One-hot encoding} of the logits. The answering parties provide $\hat{r}$ and the querying party provides $(r-\hat{r})$ to run Yao’s garbled circuit protocol~\cite{Yao:1986:GES:1382439.1382944}. They compute the argmax of the logits and transform them into one-hot representations. Each one-hot vector is split into shares $s$ and $\hat{s}$. The $s$ share is returned to the querying party and the $\hat{s}$ share is sent to the Privacy Guardian (PG). The PG is a common facilitator in these setups, i.e., a trusted third-party, and is honest-but-curious. The sum of shares $s$ and $\hat{s}$ is the one-hot encoding of the predicted label.
    \end{enumerate}
    \item \textbf{DP mechanism.} This step follows PATE to provide privacy for each teacher’s data. In PATE, Gaussian noise is added to the argmax. In \capc, Gaussian noise is added to the sum of $\hat{s}$ shares by the PG, after being collected from each of the answering parties. %At the same time, the querying party sums its $s$ values.
    \item \textbf{Noisy argmax} to compute the final label. The PG and the querying party run Yao’s garbled circuit to sum the noisy $\hat{s}$ values with the $s$ values. The result is a noisy histogram representing the number of votes for each class. The argmax of this determines which class received the maximum number of votes. This class is returned to the querying party as the final predicted label.
\end{enumerate}

\begin{algorithm}
  \caption{CaPC protocol}\label{capc-protocol}
  
  \algorithmicrequire{Querying Party QP. $x$ - query (unlabeled data item) from QP. Answering Parties AP$_1$,...,AP$_n$ with ML models $f_i(x)=y$, where $i \in \{1,...,n\}$, and $y$ is the vector of logits. Privacy Guardian PG.}
  
  \algorithmicensure{label $\ell$ for query $x$ (QP receives $\ell$ for its $x$).} 
  
  \begin{algorithmic}[1]
      \State QP encrypts $x$ to $Enc(x)$.
      \State QP sends $Enc(x)$ to AP$_1$,...,AP$_n$.
      
      \ForAll{AP$_i$}
         \State $Enc(r)_i \gets f_i(Enc(x))$
         \State Generate random $\hat{r}_i$
         \State $Enc(r_i - \hat{r}_i) \gets Enc(r_i) - \hat{r}_i$ \Comment{Enabled by Homomorphic Encryption}
         \State Send $Enc(r_i - \hat{r}_i)$ to QP 
      \EndFor
      
      \ForAll{AP$_i$ and QP} \Comment{2PC (Secure 2-Party Computation) between each AP and the QP}
         \State QP decrypts $r_i - \hat{r}_i \gets Decrypt(Enc(r_i - \hat{r}_i))$
         \State QP sends $r_i - \hat{r}_i$ to 2PC 
         \State AP$_i$ sends $\hat{r}_i$ 2PC
         \State 2PC: $r_i \gets (r_i - \hat{r}_i) + (\hat{r}_i)$
         \State 2PC: $one-hot_i \gets argmax(r_i)$
         \State 2PC: $\hat{s}_i + s \gets one-hot_i$ \Comment{Secret Sharing}
         \State AP$_i$ receives $\hat{s}_i$ from 2PC
         \State QP receives $s_i$ from 2PC
      \EndFor
      
      \ForAll{AP$_i$}
         \State Send $\hat{s}_i$ to PG.
      \EndFor
      
      \State QP: $S \gets \sum_{i=1}^{n}s_i$
      \State QP sends $S$ to 2PC
      
      \State PG: $\hat{S} \gets \sum_{i=1}^{n}\hat{s}_i$
      
      \State PG: Generate Gaussian noise $\hat{n} \gets N(0,\sigma_G)$
      
      \State PG sends $\hat{S}$ and $\hat{n}$ to 2PC
      
      \State 2PC:  $\hat{h} \gets S + \hat{S} + \hat{n}$ \Comment{Noisy histogram $\hat{h}$}
      \State 2PC: $\ell \gets argmax(\hat{h})$
      \State 2PC sends $\ell$ to QP
     
  \end{algorithmic}
\end{algorithm}


In \capc learning~\cite{capc2021iclr}, the main tool for confidentiality is secure multi-party computation (\smc)~\cite{Yao86} and homomorphic encryption. \smc is used when distrusting parties want to jointly evaluate a function on their input without revealing anything beyond the output. The \smc protocols can be divided into two main classes: (1) generic protocols, which compute any function with the~\cite{fairplay} security goal, and (2) specialized protocols, which are used to compute selected functions, for instance, the private set intersection~\cite{pinkas2020psi} or secure machine learning~\cite{mohassel2017secureml}. Even though the specialized protocols are less general, they are more efficient in terms of the execution time. Protocols in both categories use similar cryptographic building blocks, including (fully) homomorphic encryption~\cite{gentry2009fully}, secret sharing~\cite{shamir1979share}, oblivious transfer~\cite{cryptoeprint}, garbled circuits~\cite{Yao86}. Private inference can be computed in many ways and is a component of the \capc protocol that directly scales with improvements in these techniques: \capc used the HE-transformer library that uses both \smc as well as the homomorphic encryption but the private inference library can be immediately swapped with others.
